# Supplementary material for: Ultra-Broadband Microwave Frequency-Comb Generation in Superconducting Resonators
Source: arXiv:1405.7117 source file (2014-07-03)
Supplement: Supplementary file 1 [file manuscript-supplement.pdf]

# Ultra-Broadband Microwave Frequency-Comb Generation in Superconducting Resonators

## Supplemental Information

R. P. Erickson, S. R. Jefferts, and D. P. Pappas*
*National Institute of Standards and Technology, Boulder, Colorado 80305, USA*

## Supplement 1: Output Current of a Superconducting Resonator

We consider the electric circuit diagram of Figure S1.1 to model a transmission-type superconducting resonator. This is a schematic for a simple two-port resonator device held to potential $V_i(t)$ and $V_o(t)$ at the input and output ports, respectively, with input and output currents denoted by $I_i(t)$ and $I_o(t)$, respectively. There is also a leakage current $I_x(t)$ shunted to ground, save for a capacitance $C_x$. The input and output ports have capacitances $C_i$ and $C_o$, respectively. The kinetic inductance of the resonator is represented by $L_r(t)$, over which the output current $I_o(t)$ flows. The voltages $V_a(t)$ and $V_b(t)$ have been added to the diagram for reference.

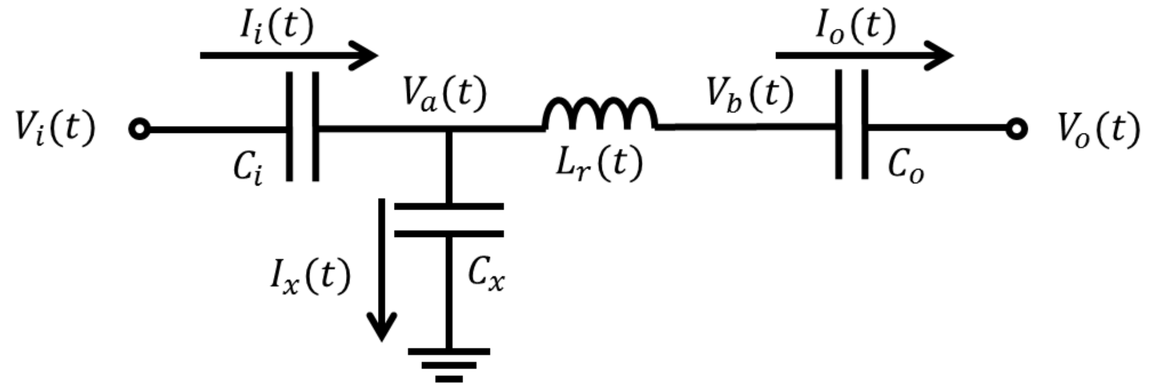


**Figure S1.1.** Circuit diagram of a lumped-element transmission line, a model of a superconducting resonator.

The voltage drops across the four electrical components at time $t$ are

$$V_i(t) - V_a(t) = \frac{1}{C_i}\int_0^t I_i(\tau)d\tau \tag{S1.1}$$

$$V_a(t) = \frac{1}{C_x}\int_0^t I_x(\tau)d\tau$$

(S1.2)

$$V_a(t) - V_b(t) = L_r(t)\frac{d}{dt}I_o(t)$$

(S1.3)

$$V_b(t) - V_o(t) = \frac{1}{C_o}\int_0^t I_o(\tau)d\tau$$

(S1.4)

The relationship between the three currents is

$$I_i(t) = I_x(t) + I_o(t)$$

(S1.5)

The above equations are manipulated to obtain a differential equation defining the output current $I_o(t)$ in terms of the driving voltages $V_i(t)$ and $V_o(t)$.

Specifically, applying (S1.2) and (S1.5) to (S1.1) gives

$$V_i(t) = \frac{1}{C_i}\int_0^t I_o(\tau)d\tau + \left(\frac{1}{C_x} + \frac{1}{C_i}\right)\int_0^t I_x(\tau)d\tau$$

(S1.6)

while applying (S1.2) and (S1.4) to (S1.3) yields

$$\frac{1}{C_x}\int_0^t I_x(\tau)d\tau - V_o(t) - \frac{1}{C_o}\int_0^t I_o(\tau)d\tau = L_r(t)\frac{d}{dt}I_o(t)$$

(S1.7)

It is convenient to multiple (S1.7) by $1/C_i + 1/C_x$ such that

$$\frac{1}{C_x}\left(\frac{1}{C_i} + \frac{1}{C_x}\right)\int_0^t I_x(\tau)d\tau - \left(\frac{1}{C_i} + \frac{1}{C_x}\right)V_o(t) - \frac{1}{C_o}\left(\frac{1}{C_i} + \frac{1}{C_x}\right)\int_0^t I_o(\tau)d\tau = \left(\frac{1}{C_i} + \frac{1}{C_x}\right)L_r(t)\frac{d}{dt}I_o(t)$$

(S1.8)

Rearranging (S1.6) to replace the integral over $I_x(\tau)$ in (S1.8) results in

$$\left(\frac{1}{C_i} + \frac{1}{C_x}\right)L_r(t)\frac{d}{dt}I_o(t) + \left[\frac{1}{C_o}\left(\frac{1}{C_i} + \frac{1}{C_x}\right) + \frac{1}{C_iC_x}\right]\int_0^t I_o(\tau)d\tau = \frac{1}{C_x}V_i(t) - \left(\frac{1}{C_i} + \frac{1}{C_x}\right)V_o(t)$$

(S1.9)

Dividing (S1.9) by $1/C_i + 1/C_x$ we obtain

$$L_r(t)\frac{d}{dt}I_o(t) + \left(\frac{1}{C_o} + \frac{1}{C_i + C_x}\right)\int_0^t I_o(\tau)d\tau = \frac{C_i}{C_i + C_x}V_i(t) - V_o(t) \equiv V(t)$$

(S1.10)

where in (S1.10) we conveniently defined an effective pump voltage

$$V(t) \equiv \frac{C_i}{C_i + C_x}V_i(t) - V_o(t)$$

(S1.11)

Differentiating (S1.10) with respect to time $t$ we arrive at

$$\frac{d}{dt}\left[L_r(t)\frac{d}{dt}I_o(t)\right] + \left(\frac{1}{C_o} + \frac{1}{C_i + C_x}\right)I_o(t) = \frac{d}{dt}V(t)$$

(S1.12)

Equation (S1.12) is the differential equation determining the output current $I_o(t)$, subject to initial boundary conditions deemed appropriate.

## Supplement 2: Nonlinear Response of a Superconducting Resonator

We present the theory of the nonlinear response of a superconducting resonator. The resonator is modeled as a lumped-element equivalent transmission line, as depicted in the circuit diagram of Figure S1.1, with capacitances at the input and output ports given by $C_i$ and $C_o$, respectively. Transmission loss is accounted for by capacitance $C_x$ to ground. Time-dependent kinetic inductance $L_r(t)$ is assumed to be the dominant source of nonlinearity via its dependence on the output current $I_o(t)$, in the manner

$$L_r(t) = L_o\left\{1 + \left[\frac{I_o(t)}{I_*}\right]^2\right\};\ L_o = \frac{\hbar R_n}{\pi\Delta}$$

(S2.1)

Here, $L_o$ is the linear inductance expressed in terms of gap parameter $\Delta$ and normal-state resistance $R_n$ of the underlying superconductor. The current $I_*$ is a scaling parameter of the expansion in powers of $I_o(t)$, where the form of the expansion is dictated by the symmetry of the film geometry.

In Supplement 1 we derived the differential equation governing $I_o(t)$ of the equivalent electric circuit, as illustrated in Figure S1.1. Defining the dimensionless amplitude $A(t) = I_o(t)/I_*$, the nonlinear second-order differential equation (S1.12) may be expressed as

$$\ddot{A}(t) + \omega_0^{(0)2} A(t) + \frac{1}{3}\frac{d^2}{dt^2} A(t)^3 = F \cos \omega t$$

(S2.2)

where the fundamental frequency of the resonator cavity is

$$\omega_0^{(0)} = \sqrt{\frac{1}{L_o}\left(\frac{1}{C_o} + \frac{1}{C_i + C_x}\right)}$$

(S2.3)

In (S2.2) we also defined the effective driving amplitude

$$F = \frac{\omega \bar{V}}{I_* L_o}$$

(S2.4)

for a pump of frequency $\omega$ and time-varying voltage $V(t) = \bar{V} \sin \omega t$. The initial boundary conditions are assumed to be $A(0) = 0$ and $\dot{A}(0) = 0$. Equation (S2.2) is similar in form to that of a Duffing oscillator, save for the $A(t)^3$ term twice differentiated with respect to time $t$. The Duffing equation is known to admit stable solutions consisting of subharmonic states whose frequencies are integer multiples of $\omega/N$,[1,2] where in this case $N$ is the integer for which $N\omega_0^{(0)}$ approximates the frequency $\omega$ of the pump. An idealized perfectly tuned pump would have frequency equal to $N$ times the fundamental.

In developing our model we purposely neglect higher normal modes of the resonator cavity, instead appealing to a lumped-element approximation. The reason for this is threefold. First is that our experimental investigations with two-tone spectroscopy have shown that higher harmonics are relatively inert with respect to the nonlinear response observed, and thus, can play no significant role. Second is that the observed resonances have extremely narrow observed linewidths, indicative of states that do not couple readily to a dissipative reservoir, unlike normal-mode excitations. Third is that the lumped-element model is sufficient to admit stable nonlinear solutions of character like that of our observations. For example, via perturbation theory, it may be shown that the weakly driven Duffing oscillator admits subharmonic states with largest amplitudes corresponding to the odd harmonics of the pump frequency, much like what we observe experimentally.[2] In the present supplement we describe via our model the onset of the subharmonic resonances that give rise to the broadband frequency response of our resonator.

## Model Calculation via Perturbation Theory

In our calculations we assume a pump of frequency $\omega$ slightly higher than $N$ integer multiples of the fundamental frequency $\omega_0^{(0)}$ of the resonator. As the pump frequency descends toward the multiple,

the pump more strongly couples to the resonator, driving the frequency of the fundamental down. Hence, the frequency of the fundamental, renormalized by strong nonlinearity, will be denoted as $\omega_0$. We will also equate the pump frequency to the value $\omega_N$, i.e., $\omega = \omega_N$, where the subscript indicates the proximity of the pump frequency to the $N$th multiple of the fundamental. The pump detuning is then the difference between $\omega_N$ and $N\omega_0$. Unlike linear resonance theory, strong coupling of pump to resonator is not dependent on proximity of pump frequency to normal mode frequency. Rather, it is the matching of phase between the natural resonance at $\omega_0$ with that of the pump feedback at $\omega_N$ that governs the strength of coupling—the closer the pump frequency is to an integer multiple of the fundamental, the stronger the coupling. In fact, the fundamental and the pump may be many octaves apart in frequency and yet couple very strongly.

In the discussion below we will adopt a perturbation theory approach, using the method of successive approximation.[3] This allows us to determine how the fundamental frequency is renormalized by the coupling of pump to resonator. It will also allow us to determine the initially strongest subharmonic resonances, and how a broadband spectrum begins to fill in at pump harmonics and corresponding sidebands as a function of increased coupling between pump and resonator.

## Approach and Zero-Order Approximation

The successive approximation is formulated as follows. We introduce a number $\epsilon \geq 0$ as a mathematical device, setting $\epsilon = 1$ at the end of calculation. We use $\epsilon$ as a formal parameter of perturbation expansion, although the actual physical perturbation parameter is $F/(\omega_N^2 - \omega_0^2)$, where in our calculations we will always assume $N > 1$. Hence, results of the perturbation theory will be most applicable when the effective pump amplitude is such that $F \ll \omega_N^2 - \omega_0^2$. This is the regime of initial coupling, i.e., weak tuning, of pump to resonator.

In this approach we expand the fundamental frequency in powers of $\epsilon$, viz.

$$\omega_0 = \omega_0^{(0)} + \epsilon\omega_0^{(1)} + \epsilon^2\omega_0^{(2)} + \cdots$$

(S2.5)

Similarly, the amplitude is expanded as

$$A(t) = A^{(0)}(t) + \epsilon A^{(1)}(t) + \epsilon^2 A^{(2)}(t) + \cdots$$

(S2.6)

The zero order of the expansion corresponds to the absence of nonlinearity. Hence, the differential equation of (S2.1) may be written as

$$\ddot{A}(t) + \omega_0^{(0)2} A(t) + \frac{1}{3}\epsilon\frac{d^2}{dt^2}A(t)^3 = F\cos\omega t$$

(S2.7)

If we include the fundamental response at $\omega_0$ and the pump feedback at $\omega_N$, as we alluded to above, then

$$A^{(0)}(t) = C_0 \cos\omega_0 t - \frac{F}{\omega_N^2 - \omega_0^2}\cos\omega_N t$$

(S2.8)

Equation (S2.8) is the solution of (S2.7) in the zero order of $\epsilon$, wherein $\omega_0 \to \omega_0^{(0)}$. In this limit we also have $C_0 = F/(\omega_N^2 - \omega_0^2)$ such that the initial boundary conditions $A^{(0)}(0) = 0$ and $\dot{A}^{(0)}(0) = 0$ are both satisfied.

## First-Order Correction

To obtain the first-order in $\epsilon$ corrections to (S2.5) and (S2.6) we first note

$$\ddot{A}^{(0)}(t) = -\omega_0^2 C_0 \cos\omega_0 t + \frac{\omega_N^2 F}{\omega_N^2 - \omega_0^2}\cos\omega_N t$$

(S2.9)

Substituting (S2.5), (S2.6), (S2.8), and (S2.9) into (S2.7), and equating terms of first order in $\epsilon$, we arrive at the constraint

$$\ddot{A}^{(1)}(t) + \omega_0^{(0)2} A^{(1)}(t) = 2\omega_0^{(0)}\omega_0^{(1)}\left(C_0\cos\omega_0 t - \frac{F}{\omega_N^2 - \omega_0^2}\cos\omega_N t\right) - \frac{1}{3}\frac{d^2}{dt^2}A^{(0)}(t)^3$$

(S2.10)

From (S2.8) and the identity

$$4\cos\alpha t\cos\beta t\cos\gamma t = \cos(\alpha+\beta-\gamma)t + \cos(\alpha-\beta+\gamma)t + \cos(\alpha-\beta-\gamma)t + \cos(\alpha+\beta+\gamma)t$$

(S2.11)

we have

$$\begin{aligned} A^{(0)}(t)^3 = \frac{1}{4}\Bigg\{ & 3C_0\left[C_0^2 + 2\frac{F^2}{(\omega_N^2-\omega_0^2)^2}\right]\cos\omega_0 t + C_0^3\cos 3\omega_0 t \\ & - 3C_0^2\frac{F}{\omega_N^2-\omega_0^2}[\cos(\omega_N - 2\omega_0)t + \cos(\omega_N + 2\omega_0)t] \\ & + 3C_0\frac{F^2}{(\omega_N^2-\omega_0^2)^2}[\cos(2\omega_N - \omega_0)t + \cos(2\omega_N + \omega_0)t] \\ & - 3\frac{F}{\omega_N^2-\omega_0^2}\left[2C_0^2 + \frac{F^2}{(\omega_N^2-\omega_0^2)^2}\right]\cos\omega_N t - \frac{F^3}{(\omega_N^2-\omega_0^2)^3}\cos 3\omega_N t\Bigg\} \end{aligned}$$

(S2.12)

and thus

$$\frac{1}{3}\frac{d^2}{dt^2}A^{(0)}(t)^3 = -\frac{1}{4}\left\{C_0\left[C_0^2 + 2\frac{F^2}{(\omega_N^2-\omega_0^2)^2}\right]\omega_0^2\cos\omega_0 t + 3C_0^3\omega_0^2\cos 3\omega_0 t\right.$$
$$- C_0^2\frac{F}{\omega_N^2-\omega_0^2}[(\omega_N-2\omega_0)^2\cos(\omega_N-2\omega_0)t + (\omega_N+2\omega_0)^2\cos(\omega_N+2\omega_0)t]$$
$$+ C_0\frac{F^2}{(\omega_N^2-\omega_0^2)^2}[(2\omega_N-\omega_0)^2\cos(2\omega_N-\omega_0)t + (2\omega_N+\omega_0)^2\cos(2\omega_N+\omega_0)t]$$
$$\left.-\frac{F}{\omega_N^2-\omega_0^2}\left[2C_0^2 + \frac{F^2}{(\omega_N^2-\omega_0^2)^2}\right]\omega_N^2\cos\omega_N t - 3\frac{F^3}{(\omega_N^2-\omega_0^2)^3}\omega_N^2\cos 3\omega_N t\right\}$$

(S2.13)

Now substituting (S2.13) into (S2.10) gives

$$\ddot{A}^{(1)}(t) + \omega_0^{(0)2}A^{(1)}(t) = 2\omega_0^{(0)}C_0\left\{\omega_0^{(1)} + \frac{1}{8}\omega_0^{(0)}\left[C_0^2 + 2\frac{F^2}{(\omega_N^2-\omega_0^2)^2}\right]\right\}\cos\omega_0 t + \frac{3}{4}\omega_0^{(0)2}C_0^3\cos 3\omega_0 t$$
$$-2\frac{F}{\omega_N^2-\omega_0^2}\left\{\omega_0^{(0)}\omega_0^{(1)} + \frac{1}{8}\omega_N^2\left[2C_0^2 + \frac{F^2}{(\omega_N^2-\omega_0^2)^2}\right]\right\}\cos\omega_N t - \frac{3}{4}\frac{\omega_N^2F^3}{(\omega_N^2-\omega_0^2)^3}\cos 3\omega_N t$$
$$-\frac{1}{4}C_0^2\frac{F}{\omega_N^2-\omega_0^2}\left\{\left[\omega_N-2\omega_0^{(0)}\right]^2\cos(\omega_N-2\omega_0)t + \left[\omega_N+2\omega_0^{(0)}\right]^2\cos(\omega_N+2\omega_0)\,t\right\}$$
$$+\frac{1}{4}C_0\frac{F^2}{(\omega_N^2-\omega_0^2)^2}\left\{\left[2\omega_N-\omega_0^{(0)}\right]^2\cos(2\omega_N-\omega_0)t + \left[2\omega_N+\omega_0^{(0)}\right]^2\cos(2\omega_N+\omega_0)t\right\}$$

(S2.14)

from which we discern a term proportional to $\cos\omega_0 t$, the secular term corresponding to the fundamental natural resonance. This term must be eliminated from (S2.14) to prevent a divergence of the perturbation expansion upon integrating to obtain $A^{(1)}(t)$. The removal of this term defines the first-order correction $\omega_0^{(1)}$, viz.

$$\omega_0^{(1)} = -\frac{1}{8}\omega_0^{(0)}\left[C_0^2 + 2\frac{F^2}{(\omega_N^2-\omega_0^2)^2}\right]$$

(S2.15)

which corresponds to a downshift of frequency with increased pump detuning. With the secular term removed, integration of (S2.14) yields the first-order amplitude correction

$$A^{(1)}(t) = -\frac{3}{32}C_0^3\cos 3\omega_0 t$$

$$+\frac{1}{4}\frac{F}{\omega_N^2-\omega_0^2}\left\{\left[\frac{2\omega_N^2-\omega_0^{(0)2}}{\omega_N^2-\omega_0^{(0)2}}\right]C_0^2+\left[\frac{\omega_N^2-2\omega_0^{(0)2}}{\omega_N^2-\omega_0^{(0)2}}\right]\frac{F^2}{(\omega_N^2-\omega_0^2)^2}\right\}\cos\omega_N t$$

$$+\frac{3}{4}\frac{F^3}{(\omega_N^2-\omega_0^2)^3}\left[\frac{\omega_N^2}{9\omega_N^2-\omega_0^{(0)2}}\right]\cos 3\omega_N t$$

$$+\frac{1}{4}C_0^2\frac{F}{\omega_N^2-\omega_0^2}\left\{\frac{\left[\omega_N-2\omega_0^{(0)}\right]^2}{\left[\omega_N-3\omega_0^{(0)}\right]\left[\omega_N-\omega_0^{(0)}\right]}\cos(\omega_N-2\omega_0)t\right.$$
$$\left.+\frac{\left[\omega_N+2\omega_0^{(0)}\right]^2}{\left[\omega_N+\omega_0^{(0)}\right]\left[\omega_N+3\omega_0^{(0)}\right]}\cos(\omega_N+2\omega_0)t\right\}$$

$$-\frac{1}{16\omega_N}C_0\frac{F^2}{(\omega_N^2-\omega_0^2)^2}\left\{\frac{\left[2\omega_N-\omega_0^{(0)}\right]^2}{\omega_N-\omega_0^{(0)}}\cos(2\omega_N-\omega_0)t+\frac{\left[2\omega_N+\omega_0^{(0)}\right]^2}{\omega_N+\omega_0^{(0)}}\cos(2\omega_N+\omega_0)t\right\}$$

(S2.16)

Equations (S2.15) and (S2.16) comprise the first-order corrections of the expansions of (S2.5) and (S2.6), respectively. Note that in (S2.16) we see the generation of third harmonics in both $\omega_0$ and $\omega_N$, and we also see the beginning of sidebands around the first and second pump harmonics. In particular, we recognize the fundamental frequency $\omega_0$ as half the free spectral range (FSR) of the broadband response—sidebands fill in at teeth separated by twice the fundamental. This may be viewed as beating between the frequencies of the natural fundamental and the pump feedback. Generally speaking, as will be seen more clearly in second order of the expansion, the sidebands of the odd (even) pump harmonics fill in, with respect to the principle resonance peak, at even (odd) multiples of the fundamental frequency. However, only the odd principle resonance peaks appear, i.e., the odd harmonics of the pump frequency; the even harmonics are absent though their corresponding sidebands begin to form. These selection rules are governed by (S2.11), and ultimately by the symmetry of the film geometry, which dictates the expansion of the kinetic inductance of (S2.1) in specific powers of $I_o(t)$.

## Second-Order Correction

If we continue the expansion of (S2.5) and (S2.6) applied to (S2.7) and equate terms in $\epsilon^2$ we find the constraint governing the second-order correction, which we may express as

$$\ddot{A}^{(2)}(t)+\omega_0^{(0)2}A^{(2)}(t)=\left[\omega_0^{(1)2}+2\omega_0^{(0)}\omega_0^{(2)}\right]\left(C_0\cos\omega_0 t-\frac{F}{\omega_N^2-\omega_0^2}\cos\omega_N t\right)$$

$$+\frac{1}{2}\omega_0^{(1)}\Bigg(\omega_0^{(0)}C_0\left[C_0^2+2\frac{F^2}{(\omega_N^2-\omega_0^2)^2}\right]\cos\omega_0 t+3\omega_0^{(0)}C_0^3\cos 3\omega_0 t$$

$$+2C_0^2\frac{F}{\omega_N^2-\omega_0^2}\left\{\left[\omega_N-2\omega_0^{(0)}\right]\cos(\omega_N-2\omega_0)t-\left[\omega_N+2\omega_0^{(0)}\right]\cos(\omega_N+2\omega_0)t\right\}$$

$$-C_0\frac{F^2}{(\omega_N^2-\omega_0^2)^2}\left\{\left[2\omega_N-\omega_0^{(0)}\right]\cos(2\omega_N-\omega_0)t-\left[2\omega_N+\omega_0^{(0)}\right]\cos(2\omega_N+\omega_0)t\right\}\Bigg)$$

$$-\frac{d^2}{dt^2}\left[A^{(0)}(t)^2A^{(1)}(t)\right]$$

(S2.17)

Here, $\omega_0^{(1)}$ and $A^{(1)}(t)$ are the corrections we obtained in first order, as given by (S2.15) and (S2.16), respectively. Equation (S2.17) consists of frequency corrections to both zero and first order amplitudes as well as the second-order nonlinearity, which involves the second derivative in time of the terms

$$A^{(0)}(t)^2A^{(1)}(t)=\left[C_0^2\cos^2\omega_0 t-2C_0\frac{F}{\omega_N^2-\omega_0^2}\cos\omega_0 t\cos\omega_N t+\frac{F^2}{(\omega_N^2-\omega_0^2)^2}\cos^2\omega_N t\right]$$

$$\times\Bigg(-\frac{3}{32}C_0^3\cos 3\omega_0 t+\frac{1}{4}\frac{F}{\omega_N^2-\omega_0^2}\left\{\left[\frac{2\omega_N^2-\omega_0^{(0)2}}{\omega_N^2-\omega_0^{(0)2}}\right]C_0^2+\left[\frac{\omega_N^2-2\omega_0^{(0)2}}{\omega_N^2-\omega_0^{(0)2}}\right]\frac{F^2}{(\omega_N^2-\omega_0^2)^2}\right\}\cos\omega_N t$$

$$+\frac{3}{4}\frac{F^3}{(\omega_N^2-\omega_0^2)^3}\left[\frac{\omega_N^2}{9\omega_N^2-\omega_0^{(0)2}}\right]\cos 3\omega_N t$$

$$+\frac{1}{4}C_0^2\frac{F}{\omega_N^2-\omega_0^2}\left\{\frac{\left[\omega_N-2\omega_0^{(0)}\right]^2}{\left[\omega_N-3\omega_0^{(0)}\right]\left[\omega_N-\omega_0^{(0)}\right]}\cos(\omega_N-2\omega_0)t\right.$$

$$\left.+\frac{\left[\omega_N+2\omega_0^{(0)}\right]^2}{\left[\omega_N+\omega_0^{(0)}\right]\left[\omega_N+3\omega_0^{(0)}\right]}\cos(\omega_N+2\omega_0)t\right\}$$

$$-\frac{1}{16\omega_N}C_0\frac{F^2}{(\omega_N^2-\omega_0^2)^2}\left\{\frac{\left[2\omega_N-\omega_0^{(0)}\right]^2}{\omega_N-\omega_0^{(0)}}\cos(2\omega_N-\omega_0)t+\frac{\left[2\omega_N+\omega_0^{(0)}\right]^2}{\omega_N+\omega_0^{(0)}}\cos(2\omega_N+\omega_0)t\right\}\Bigg)$$

(S2.18)

If the factors of (S2.18) are distributed and the identity of (S2.11) is used then terms of like harmonic may be grouped together. After some tedious algebra the result may be written as

$A^{(0)}(t)^2A^{(1)}(t)=$

$$
\begin{aligned}
&-\frac{1}{8}C_0\left(\frac{3}{16}C_0^4+C_0^2\frac{F^2}{(\omega_N^2-\omega_0^2)^2}\left\{2\left[\frac{2\omega_N^2-\omega_0^{(0)2}}{\omega_N^2-\omega_0^{(0)2}}\right]+\frac{\left[\omega_N-2\omega_0^{(0)}\right]^2}{\left[\omega_N-3\omega_0^{(0)}\right]\left[\omega_N-\omega_0^{(0)}\right]}\right.\right.\\
&\qquad\left.+\frac{\left[\omega_N+2\omega_0^{(0)}\right]^2}{\left[\omega_N+\omega_0^{(0)}\right]\left[\omega_N+3\omega_0^{(0)}\right]}\right\}\\
&\qquad+\frac{1}{2}\frac{F^4}{(\omega_N^2-\omega_0^2)^4}\left\{4\left[\frac{\omega_N^2-2\omega_0^{(0)2}}{\omega_N^2-\omega_0^{(0)2}}\right]+\frac{\left[2\omega_N-\omega_0^{(0)}\right]^2}{2\omega_N\left[2\omega_N-2\omega_0^{(0)}\right]}\right.\\
&\qquad\left.\left.+\frac{\left[2\omega_N+\omega_0^{(0)}\right]^2}{2\omega_N\left[2\omega_N+2\omega_0^{(0)}\right]}\right\}\right)\cos\omega_0 t
\end{aligned}
$$

$$
\begin{aligned}
&-\frac{1}{8}C_0^3\left(\frac{3}{8}C_0^2+\frac{F^2}{(\omega_N^2-\omega_0^2)^2}\left\{1+\frac{\left[\omega_N-2\omega_0^{(0)}\right]^2}{\left[\omega_N-3\omega_0^{(0)}\right]\left[\omega_N-\omega_0^{(0)}\right]}+\frac{\left[\omega_N+2\omega_0^{(0)}\right]^2}{\left[\omega_N+\omega_0^{(0)}\right]\left[\omega_N+3\omega_0^{(0)}\right]}\right\}\right)\cos 3\omega_0 t\\
&\qquad-\frac{3}{128}C_0^5\cos 5\omega_0 t
\end{aligned}
$$

$$
\begin{aligned}
&+\frac{1}{16}\frac{F}{\omega_N^2-\omega_0^2}\left(C_0^4\left\{2\left[\frac{2\omega_N^2-\omega_0^{(0)2}}{\omega_N^2-\omega_0^{(0)2}}\right]+\frac{\left[\omega_N-2\omega_0^{(0)}\right]^2}{\left[\omega_N-3\omega_0^{(0)}\right]\left[\omega_N-\omega_0^{(0)}\right]}+\frac{\left[\omega_N+2\omega_0^{(0)}\right]^2}{\left[\omega_N+\omega_0^{(0)}\right]\left[\omega_N+3\omega_0^{(0)}\right]}\right\}\right.\\
&\qquad+C_0^2\frac{F^2}{(\omega_N^2-\omega_0^2)^2}\left\{2\left[\frac{\omega_N^2-2\omega_0^{(0)2}}{\omega_N^2-\omega_0^{(0)2}}\right]+3\left[\frac{2\omega_N^2-\omega_0^{(0)2}}{\omega_N^2-\omega_0^{(0)2}}\right]+\frac{\left[2\omega_N-\omega_0^{(0)}\right]^2}{\omega_N\left[2\omega_N-2\omega_0^{(0)}\right]}\right.\\
&\qquad\left.\left.+\frac{\left[2\omega_N+\omega_0^{(0)}\right]^2}{\omega_N\left[2\omega_N+2\omega_0^{(0)}\right]}\right\}+3\frac{F^4}{(\omega_N^2-\omega_0^2)^4}\left\{\left[\frac{\omega_N^2-2\omega_0^{(0)2}}{\omega_N^2-\omega_0^{(0)2}}\right]+\left[\frac{\omega_N^2}{9\omega_N^2-\omega_0^{(0)2}}\right]\right\}\right)\cos\omega_N t
\end{aligned}
$$

$$
\begin{aligned}
&+\frac{1}{16}\frac{F^3}{(\omega_N^2-\omega_0^2)^3}\left(C_0^2\left\{6\left[\frac{\omega_N^2}{9\omega_N^2-\omega_0^{(0)2}}\right]+\left[\frac{2\omega_N^2-\omega_0^{(0)2}}{\omega_N^2-\omega_0^{(0)2}}\right]+\frac{\left[2\omega_N-\omega_0^{(0)}\right]^2}{\omega_N\left[2\omega_N-2\omega_0^{(0)}\right]}+\frac{\left[2\omega_N+\omega_0^{(0)}\right]^2}{\omega_N\left[2\omega_N+2\omega_0^{(0)}\right]}\right\}\right.\\
&\qquad\left.+\frac{F^2}{(\omega_N^2-\omega_0^2)^2}\left\{6\left[\frac{\omega_N^2}{9\omega_N^2-\omega_0^{(0)2}}\right]+\left[\frac{\omega_N^2-2\omega_0^{(0)2}}{\omega_N^2-\omega_0^{(0)2}}\right]\right\}\right)\cos 3\omega_N t
\end{aligned}
$$

$$
+\frac{3}{16}\frac{F^5}{(\omega_N^2-\omega_0^2)^5}\left[\frac{\omega_N^2}{9\omega_N^2-\omega_0^{(0)2}}\right]\cos 5\omega_N t
$$

$$+\frac{1}{16}C_0^2\frac{F}{\omega_N^2-\omega_0^2}\left(C_0^2\left\{\frac{3}{4}+\left[\frac{2\omega_N^2-\omega_0^{(0)2}}{\omega_N^2-\omega_0^{(0)2}}\right]+2\frac{\left[\omega_N-2\omega_0^{(0)}\right]^2}{\left[\omega_N-3\omega_0^{(0)}\right]\left[\omega_N-\omega_0^{(0)}\right]}\right\}\right.$$

$$+\frac{F^2}{(\omega_N^2-\omega_0^2)^2}\left\{\left[\frac{\omega_N^2-2\omega_0^{(0)2}}{\omega_N^2-\omega_0^{(0)2}}\right]+\frac{\left[2\omega_N-\omega_0^{(0)}\right]^2}{\omega_N\left[2\omega_N-2\omega_0^{(0)}\right]}+2\frac{\left[\omega_N-2\omega_0^{(0)}\right]^2}{\left[\omega_N-3\omega_0^{(0)}\right]\left[\omega_N-\omega_0^{(0)}\right]}\right.$$

$$\left.\left.+\frac{\left[\omega_N+2\omega_0^{(0)}\right]^2}{\left[\omega_N+\omega_0^{(0)}\right]\left[\omega_N+3\omega_0^{(0)}\right]}\right\}\right)\cos(\omega_N-2\omega_0)t$$

$$+\frac{1}{16}C_0^2\frac{F}{\omega_N^2-\omega_0^2}\left(C_0^2\left\{\frac{3}{4}+\left[\frac{2\omega_N^2-\omega_0^{(0)2}}{\omega_N^2-\omega_0^{(0)2}}\right]+2\frac{\left[\omega_N+2\omega_0^{(0)}\right]^2}{\left[\omega_N+\omega_0^{(0)}\right]\left[\omega_N+3\omega_0^{(0)}\right]}\right\}\right.$$

$$+\frac{F^2}{(\omega_N^2-\omega_0^2)^2}\left\{\left[\frac{\omega_N^2-2\omega_0^{(0)2}}{\omega_N^2-\omega_0^{(0)2}}\right]+\frac{\left[2\omega_N+\omega_0^{(0)}\right]^2}{\omega_N\left[2\omega_N+2\omega_0^{(0)}\right]}+2\frac{\left[\omega_N+2\omega_0^{(0)}\right]^2}{\left[\omega_N+\omega_0^{(0)}\right]\left[\omega_N+3\omega_0^{(0)}\right]}\right.$$

$$\left.\left.+\frac{\left[\omega_N-2\omega_0^{(0)}\right]^2}{\left[\omega_N-3\omega_0^{(0)}\right]\left[\omega_N-\omega_0^{(0)}\right]}\right\}\right)\cos(\omega_N+2\omega_0)t$$

$$+\frac{1}{16}C_0^4\frac{F}{\omega_N^2-\omega_0^2}\left\{\frac{3}{4}+\frac{\left[\omega_N-2\omega_0^{(0)}\right]^2}{\left[\omega_N-3\omega_0^{(0)}\right]\left[\omega_N-\omega_0^{(0)}\right]}\right\}\cos(\omega_N-4\omega_0)t$$

$$+\frac{1}{16}C_0^4\frac{F}{\omega_N^2-\omega_0^2}\left\{\frac{3}{4}+\frac{\left[\omega_N+2\omega_0^{(0)}\right]^2}{\left[\omega_N+\omega_0^{(0)}\right]\left[\omega_N+3\omega_0^{(0)}\right]}\right\}\cos(\omega_N+4\omega_0)\,t$$

$$-\frac{1}{16}C_0\frac{F^2}{(\omega_N^2-\omega_0^2)^2}\left(2C_0^2\left\{\left[\frac{2\omega_N^2-\omega_0^{(0)2}}{\omega_N^2-\omega_0^{(0)2}}\right]+\frac{\left[\omega_N-2\omega_0^{(0)}\right]^2}{\left[\omega_N-3\omega_0^{(0)}\right]\left[\omega_N-\omega_0^{(0)}\right]}+\frac{\left[2\omega_N-\omega_0^{(0)}\right]^2}{2\omega_N\left[2\omega_N-2\omega_0^{(0)}\right]}\right.\right.$$

$$\left.+\frac{\left[2\omega_N+\omega_0^{(0)}\right]^2}{4\omega_N\left[2\omega_N+2\omega_0^{(0)}\right]}\right\}$$

$$+2\frac{F^2}{(\omega_N^2-\omega_0^2)^2}\left\{\left[\frac{\omega_N^2-2\omega_0^{(0)2}}{\omega_N^2-\omega_0^{(0)2}}\right]+3\left[\frac{\omega_N^2}{9\omega_N^2-\omega_0^{(0)2}}\right]\right.$$

$$\left.\left.+\frac{\left[2\omega_N-\omega_0^{(0)}\right]^2}{2\omega_N\left[2\omega_N-2\omega_0^{(0)}\right]}\right\}\right)\cos(2\omega_N-\omega_0)t$$

$$-\frac{1}{16}C_0\frac{F^2}{(\omega_N^2-\omega_0^2)^2}\left(2C_0^2\left\{\left[\frac{2\omega_N^2-\omega_0^{(0)2}}{\omega_N^2-\omega_0^{(0)2}}\right]+\frac{\left[\omega_N+2\omega_0^{(0)}\right]^2}{\left[\omega_N+\omega_0^{(0)}\right]\left[\omega_N+3\omega_0^{(0)}\right]}+\frac{\left[2\omega_N+\omega_0^{(0)}\right]^2}{2\omega_N\left[2\omega_N+2\omega_0^{(0)}\right]}\right.\right.$$

$$\left.+\frac{\left[2\omega_N-\omega_0^{(0)}\right]^2}{4\omega_N\left[2\omega_N-2\omega_0^{(0)}\right]}\right\}$$

$$+2\frac{F^2}{(\omega_N^2-\omega_0^2)^2}\left\{\left[\frac{\omega_N^2-2\omega_0^{(0)2}}{\omega_N^2-\omega_0^{(0)2}}\right]+3\left[\frac{\omega_N^2}{9\omega_N^2-\omega_0^{(0)2}}\right]\right.$$

$$\left.\left.+\frac{\left[2\omega_N+\omega_0^{(0)}\right]^2}{2\omega_N\left[2\omega_N+2\omega_0^{(0)}\right]}\right\}\right)\cos(2\omega_N+\omega_0)t$$

$$-\frac{1}{16}C_0^3\frac{F^2}{(\omega_N^2-\omega_0^2)^2}\left\{\frac{3}{8}+\frac{\left[2\omega_N-\omega_0^{(0)}\right]^2}{2\omega_N\left[2\omega_N-2\omega_0^{(0)}\right]}+2\frac{\left[\omega_N-2\omega_0^{(0)}\right]^2}{\left[\omega_N-3\omega_0^{(0)}\right]\left[\omega_N-\omega_0^{(0)}\right]}\right\}\cos(2\omega_N-3\omega_0)t$$

$$-\frac{1}{16}C_0^3\frac{F^2}{(\omega_N^2-\omega_0^2)^2}\left\{\frac{3}{8}+\frac{\left[2\omega_N+\omega_0^{(0)}\right]^2}{2\omega_N\left[2\omega_N+2\omega_0^{(0)}\right]}+2\frac{\left[\omega_N+2\omega_0^{(0)}\right]^2}{\left[\omega_N+\omega_0^{(0)}\right]\left[\omega_N+3\omega_0^{(0)}\right]}\right\}\cos(2\omega_N+3\omega_0)t$$

$$+\frac{1}{16}C_0^2\frac{F^3}{(\omega_N^2-\omega_0^2)^3}\left\{3\left[\frac{\omega_N^2}{9\omega_N^2-\omega_0^{(0)2}}\right]+\frac{\left[\omega_N-2\omega_0^{(0)}\right]^2}{\left[\omega_N-3\omega_0^{(0)}\right]\left[\omega_N-\omega_0^{(0)}\right]}\right.$$

$$\left.+\frac{\left[2\omega_N-\omega_0^{(0)}\right]^2}{\omega_N\left[2\omega_N-2\omega_0^{(0)}\right]}\right\}\cos(3\omega_N-2\omega_0)t$$

$$+\frac{1}{16}C_0^2\frac{F^3}{(\omega_N^2-\omega_0^2)^3}\left\{3\left[\frac{\omega_N^2}{9\omega_N^2-\omega_0^{(0)2}}\right]+\frac{\left[\omega_N+2\omega_0^{(0)}\right]^2}{\left[\omega_N+\omega_0^{(0)}\right]\left[\omega_N+3\omega_0^{(0)}\right]}\right.$$

$$\left.+\frac{\left[2\omega_N+\omega_0^{(0)}\right]^2}{\omega_N\left[2\omega_N+2\omega_0^{(0)}\right]}\right\}\cos(3\omega_N+2\omega_0)t$$

$$-\frac{3}{8}C_0\frac{F^4}{(\omega_N^2-\omega_0^2)^4}\left\{\left[\frac{\omega_N^2}{9\omega_N^2-\omega_0^{(0)2}}\right]+\frac{\left[2\omega_N-\omega_0^{(0)}\right]^2}{4\omega_N\left[2\omega_N-2\omega_0^{(0)}\right]}\right\}\cos(4\omega_N-\omega_0)t$$

$$-\frac{3}{8}C_0\frac{F^4}{(\omega_N^2-\omega_0^2)^4}\left\{\left[\frac{\omega_N^2}{9\omega_N^2-\omega_0^{(0)2}}\right]+\frac{\left[2\omega_N+\omega_0^{(0)}\right]^2}{4\omega_N\left[2\omega_N+2\omega_0^{(0)}\right]}\right\}\cos(4\omega_N+\omega_0)t$$

(S2.19)

Though a lengthy formula, it is straightforward to differentiate (S2.19) twice with respect to the time variable $t$ and apply the result to (S2.17). In so doing, and incorporating the correction of (S2.15), we obtain

$$\ddot{A}^{(2)}(t)+\omega_0^{(0)2}A^{(2)}(t)=$$

$$2C_0\omega_0^{(0)}\left(\omega_0^{(2)}-\frac{9}{256}C_0^4\omega_0^{(0)}\right.$$

$$-\frac{1}{32}C_0^2\frac{\omega_0^{(0)}F^2}{(\omega_N^2-\omega_0^2)^2}\left\{3+4\left[\frac{2\omega_N^2-\omega_0^{(0)2}}{\omega_N^2-\omega_0^{(0)2}}\right]+2\frac{\left[\omega_N-2\omega_0^{(0)}\right]^2}{\left[\omega_N-3\omega_0^{(0)}\right]\left[\omega_N-\omega_0^{(0)}\right]}\right.$$

$$\left.+2\frac{\left[\omega_N+2\omega_0^{(0)}\right]^2}{\left[\omega_N+\omega_0^{(0)}\right]\left[\omega_N+3\omega_0^{(0)}\right]}\right\}$$

$$-\frac{1}{32}\frac{\omega_0^{(0)}F^4}{(\omega_N^2-\omega_0^2)^4}\left\{3+4\left[\frac{\omega_N^2-2\omega_0^{(0)2}}{\omega_N^2-\omega_0^{(0)2}}\right]+\frac{\left[2\omega_N-\omega_0^{(0)}\right]^2}{4\omega_N\left[\omega_N-\omega_0^{(0)}\right]}\right.$$

$$\left.\left.+\frac{\left[2\omega_N+\omega_0^{(0)}\right]^2}{4\omega_N\left[\omega_N+\omega_0^{(0)}\right]}\right\}\right)\cos\omega_0 t$$

$$-\frac{3}{8}C_0^3\omega_0^{(0)2}\left(\frac{25}{8}C_0^2\right.$$

$$+\frac{F^2}{(\omega_N^2-\omega_0^2)^2}\left\{4+\frac{3\left[\omega_N-2\omega_0^{(0)}\right]^2}{\left[\omega_N-3\omega_0^{(0)}\right]\left[\omega_N-\omega_0^{(0)}\right]}\right.$$

$$\left.\left.+\frac{3\left[\omega_N+2\omega_0^{(0)}\right]^2}{\left[\omega_N+\omega_0^{(0)}\right]\left[\omega_N+3\omega_0^{(0)}\right]}\right\}\right)\cos 3\omega_0 t-\frac{75}{128}C_0^5\omega_0^{(0)2}\cos 5\omega_0 t$$

$$-\frac{F}{\omega_N^2-\omega_0^2}\Bigg(2\omega_0^{(0)}\omega_0^{(2)}+\frac{1}{64}\omega_0^{(0)2}\left[C_0^2+2\frac{F^2}{(\omega_N^2-\omega_0^2)^2}\right]^2$$

$$-\frac{1}{16}C_0^4\omega_N^2\Bigg\{2\left[\frac{2\omega_N^2-\omega_0^{(0)2}}{\omega_N^2-\omega_0^{(0)2}}\right]+\frac{\left[\omega_N-2\omega_0^{(0)}\right]^2}{\left[\omega_N-3\omega_0^{(0)}\right]\left[\omega_N-\omega_0^{(0)}\right]}$$

$$+\frac{\left[\omega_N+2\omega_0^{(0)}\right]^2}{\left[\omega_N+\omega_0^{(0)}\right]\left[\omega_N+3\omega_0^{(0)}\right]}\Bigg\}$$

$$-\frac{1}{16}C_0^2\frac{\omega_N^2F^2}{(\omega_N^2-\omega_0^2)^2}\Bigg\{2\left[\frac{\omega_N^2-2\omega_0^{(0)2}}{\omega_N^2-\omega_0^{(0)2}}\right]+3\left[\frac{2\omega_N^2-\omega_0^{(0)2}}{\omega_N^2-\omega_0^{(0)2}}\right]+\frac{\left[2\omega_N-\omega_0^{(0)}\right]^2}{\omega_N\left[2\omega_N-2\omega_0^{(0)}\right]}$$

$$+\frac{\left[2\omega_N+\omega_0^{(0)}\right]^2}{\omega_N\left[2\omega_N+2\omega_0^{(0)}\right]}\Bigg\}-\frac{3}{16}\frac{\omega_N^2F^4}{(\omega_N^2-\omega_0^2)^4}\Bigg\{\left[\frac{\omega_N^2-2\omega_0^{(0)2}}{\omega_N^2-\omega_0^{(0)2}}\right]+\left[\frac{\omega_N^2}{9\omega_N^2-\omega_0^{(0)2}}\right]\Bigg\}\Bigg)\cos\omega_N t$$

$$+\frac{9}{16}\frac{F^3}{(\omega_N^2-\omega_0^2)^3}\omega_N^2\Bigg(C_0^2\Bigg\{6\left[\frac{\omega_N^2}{9\omega_N^2-\omega_0^{(0)2}}\right]+\left[\frac{2\omega_N^2-\omega_0^{(0)2}}{\omega_N^2-\omega_0^{(0)2}}\right]+\frac{\left[2\omega_N-\omega_0^{(0)}\right]^2}{\omega_N\left[2\omega_N-2\omega_0^{(0)}\right]}$$

$$+\frac{\left[2\omega_N+\omega_0^{(0)}\right]^2}{\omega_N\left[2\omega_N+2\omega_0^{(0)}\right]}\Bigg\}+\frac{F^2}{(\omega_N^2-\omega_0^2)^2}\Bigg\{6\left[\frac{\omega_N^2}{9\omega_N^2-\omega_0^{(0)2}}\right]+\left[\frac{\omega_N^2-2\omega_0^{(0)2}}{\omega_N^2-\omega_0^{(0)2}}\right]\Bigg\}\Bigg)\cos 3\omega_N t$$

$$+\frac{75}{16}\frac{F^5}{(\omega_N^2-\omega_0^2)^5}\left[\frac{\omega_N^4}{9\omega_N^2-\omega_0^{(0)2}}\right]\cos 5\omega_N t$$

$$-\frac{1}{16}C_0^2\frac{F}{\omega_N^2-\omega_0^2}\Bigg(2\omega_0^{(0)}\left[\omega_N-2\omega_0^{(0)}\right]\left[C_0^2+2\frac{F^2}{(\omega_N^2-\omega_0^2)^2}\right]$$

$$-C_0^2\left[\omega_N-2\omega_0^{(0)}\right]^2\Bigg\{\frac{3}{4}+\left[\frac{2\omega_N^2-\omega_0^{(0)2}}{\omega_N^2-\omega_0^{(0)2}}\right]+2\frac{\left[\omega_N-2\omega_0^{(0)}\right]^2}{\left[\omega_N-3\omega_0^{(0)}\right]\left[\omega_N-\omega_0^{(0)}\right]}\Bigg\}$$

$$-\frac{F^2}{(\omega_N^2-\omega_0^2)^2}\left[\omega_N-2\omega_0^{(0)}\right]^2\Bigg\{\left[\frac{\omega_N^2-2\omega_0^{(0)2}}{\omega_N^2-\omega_0^{(0)2}}\right]+\frac{\left[2\omega_N-\omega_0^{(0)}\right]^2}{2\omega_N\left[\omega_N-\omega_0^{(0)}\right]}$$

$$+2\frac{\left[\omega_N-2\omega_0^{(0)}\right]^2}{\left[\omega_N-3\omega_0^{(0)}\right]\left[\omega_N-\omega_0^{(0)}\right]}+\frac{\left[\omega_N+2\omega_0^{(0)}\right]^2}{\left[\omega_N+\omega_0^{(0)}\right]\left[\omega_N+3\omega_0^{(0)}\right]}\Bigg\}\Bigg)\cos(\omega_N-2\omega_0)t$$

$$+\frac{1}{16}C_0^2\frac{F}{\omega_N^2-\omega_0^2}\left(2\omega_0^{(0)}\left[\omega_N+2\omega_0^{(0)}\right]\left[C_0^2+2\frac{F^2}{(\omega_N^2-\omega_0^2)^2}\right]\right.$$

$$+C_0^2\left[\omega_N+2\omega_0^{(0)}\right]^2\left\{\frac{3}{4}+\left[\frac{2\omega_N^2-\omega_0^{(0)2}}{\omega_N^2-\omega_0^{(0)2}}\right]+2\frac{\left[\omega_N+2\omega_0^{(0)}\right]^2}{\left[\omega_N+\omega_0^{(0)}\right]\left[\omega_N+3\omega_0^{(0)}\right]}\right\}$$

$$+\frac{F^2}{(\omega_N^2-\omega_0^2)^2}\left[\omega_N+2\omega_0^{(0)}\right]^2\left\{\left[\frac{\omega_N^2-2\omega_0^{(0)2}}{\omega_N^2-\omega_0^{(0)2}}\right]+\frac{\left[2\omega_N+\omega_1^{(0)}\right]^2}{2\omega_N\left[\omega_N+\omega_1^{(0)}\right]}\right.$$

$$\left.\left.+2\frac{\left[\omega_N+2\omega_0^{(0)}\right]^2}{\left[\omega_N+\omega_0^{(0)}\right]\left[\omega_N+3\omega_0^{(0)}\right]}+\frac{\left[\omega_N-2\omega_0^{(0)}\right]^2}{\left[\omega_N-3\omega_0^{(0)}\right]\left[\omega_N-\omega_0^{(0)}\right]}\right\}\right)\cos(\omega_N+2\omega_0)t$$

$$+\frac{1}{16}C_0^4\left[\omega_N-4\omega_0^{(0)}\right]^2\frac{F}{\omega_N^2-\omega_0^2}\left\{\frac{3}{4}+\frac{\left[\omega_N-2\omega_0^{(0)}\right]^2}{\left[\omega_N-3\omega_0^{(0)}\right]\left[\omega_N-\omega_0^{(0)}\right]}\right\}\cos(\omega_N-4\omega_0)t$$

$$+\frac{1}{16}C_0^4\left[\omega_N+4\omega_0^{(0)}\right]^2\frac{F}{\omega_N^2-\omega_0^2}\left\{\frac{3}{4}+\frac{\left[\omega_N+2\omega_0^{(0)}\right]^2}{\left[\omega_N+\omega_0^{(0)}\right]\left[\omega_N+3\omega_0^{(0)}\right]}\right\}\cos(\omega_N+4\omega_0)\,t$$

$$+\frac{1}{16}C_0\frac{F^2}{(\omega_N^2-\omega_0^2)^2}\left(\omega_0^{(0)}\left[2\omega_N-\omega_0^{(0)}\right]\left[C_0^2+2\frac{F^2}{(\omega_N^2-\omega_0^2)^2}\right]\right.$$

$$-2C_0^2\left[2\omega_N-\omega_0^{(0)}\right]^2\left\{\left[\frac{2\omega_N^2-\omega_0^{(0)2}}{\omega_N^2-\omega_0^{(0)2}}\right]+\frac{\left[\omega_N-2\omega_0^{(0)}\right]^2}{\left[\omega_N-3\omega_0^{(0)}\right]\left[\omega_N-\omega_0^{(0)}\right]}\right.$$

$$\left.+\frac{\left[2\omega_N-\omega_0^{(0)}\right]^2}{4\omega_N\left[\omega_N-\omega_0^{(0)}\right]}+\frac{\left[2\omega_N+\omega_0^{(0)}\right]^2}{8\omega_N\left[\omega_N+\omega_0^{(0)}\right]}\right\}$$

$$-2\frac{F^2}{(\omega_N^2-\omega_0^2)^2}\left[2\omega_N-\omega_0^{(0)}\right]^2\left\{\left[\frac{\omega_N^2-2\omega_0^{(0)2}}{\omega_N^2-\omega_0^{(0)2}}\right]+3\left[\frac{\omega_N^2}{9\omega_N^2-\omega_0^{(0)2}}\right]\right.$$

$$\left.\left.+\frac{\left[2\omega_N-\omega_0^{(0)}\right]^2}{4\omega_N\left[\omega_N-\omega_0^{(0)}\right]}\right\}\right)\cos(2\omega_N-\omega_0)t$$

$$-\frac{1}{16}C_0\frac{F^2}{(\omega_N^2-\omega_0^2)^2}\left(\omega_0^{(0)}\left[2\omega_N+\omega_0^{(0)}\right]\left[C_0^2+2\frac{F^2}{(\omega_N^2-\omega_0^2)^2}\right]\right.$$

$$+2C_0^2\left[2\omega_N+\omega_0^{(0)}\right]^2\left\{\left[\frac{2\omega_N^2-\omega_0^{(0)2}}{\omega_N^2-\omega_0^{(0)2}}\right]+\frac{\left[\omega_N+2\omega_0^{(0)}\right]^2}{\left[\omega_N+\omega_0^{(0)}\right]\left[\omega_N+3\omega_0^{(0)}\right]}\right.$$

$$\left.+\frac{\left[2\omega_N+\omega_0^{(0)}\right]^2}{4\omega_N\left[\omega_N+\omega_0^{(0)}\right]}+\frac{\left[2\omega_N-\omega_0^{(0)}\right]^2}{8\omega_N\left[\omega_N-\omega_0^{(0)}\right]}\right\}$$

$$+2\frac{F^2}{(\omega_N^2-\omega_0^2)^2}\left[2\omega_N+\omega_0^{(0)}\right]^2\left\{\left[\frac{\omega_N^2-2\omega_0^{(0)2}}{\omega_N^2-\omega_0^{(0)2}}\right]+3\left[\frac{\omega_N^2}{9\omega_N^2-\omega_0^{(0)2}}\right]\right.$$

$$\left.\left.+\frac{\left[2\omega_N+\omega_0^{(0)}\right]^2}{4\omega_N\left[\omega_N+\omega_0^{(0)}\right]}\right\}\right)\cos(2\omega_N+\omega_0)t$$

$$-\frac{1}{16}C_0^3\frac{F^2}{(\omega_N^2-\omega_0^2)^2}\left[2\omega_N-3\omega_0^{(0)}\right]^2\left\{\frac{3}{8}+\frac{\left[2\omega_N-\omega_0^{(0)}\right]^2}{4\omega_N\left[\omega_N-\omega_0^{(0)}\right]}\right.$$

$$\left.+2\frac{\left[\omega_N-2\omega_0^{(0)}\right]^2}{\left[\omega_N-3\omega_0^{(0)}\right]\left[\omega_N-\omega_0^{(0)}\right]}\right\}\cos(2\omega_N-3\omega_0)t$$

$$-\frac{1}{16}C_0^3\frac{F^2}{(\omega_N^2-\omega_0^2)^2}\left[2\omega_N+3\omega_0^{(0)}\right]^2\left\{\frac{3}{8}+\frac{\left[2\omega_N+\omega_0^{(0)}\right]^2}{4\omega_N\left[\omega_N+\omega_0^{(0)}\right]}\right.$$

$$\left.+2\frac{\left[\omega_N+2\omega_0^{(0)}\right]^2}{\left[\omega_N+\omega_0^{(0)}\right]\left[\omega_N+3\omega_0^{(0)}\right]}\right\}\cos(2\omega_N+3\omega_0)t$$

$$+\frac{1}{16}C_0^2\frac{F^3}{(\omega_N^2-\omega_0^2)^3}\left[3\omega_N-2\omega_0^{(0)}\right]^2\left\{3\left[\frac{\omega_N^2}{9\omega_N^2-\omega_0^{(0)2}}\right]+\frac{\left[\omega_N-2\omega_0^{(0)}\right]^2}{\left[\omega_N-3\omega_0^{(0)}\right]\left[\omega_N-\omega_0^{(0)}\right]}\right.$$

$$\left.+\frac{\left[2\omega_N-\omega_0^{(0)}\right]^2}{2\omega_N\left[\omega_N-\omega_0^{(0)}\right]}\right\}\cos(3\omega_N-2\omega_0)t$$

$$+\frac{1}{16}C_0^2\frac{F^3}{(\omega_N^2-\omega_0^2)^3}\left[3\omega_N+2\omega_0^{(0)}\right]^2\left\{3\left[\frac{\omega_N^2}{9\omega_N^2-\omega_0^{(0)2}}\right]+\frac{\left[\omega_N+2\omega_0^{(0)}\right]^2}{\left[\omega_N+\omega_0^{(0)}\right]\left[\omega_N+3\omega_0^{(0)}\right]}\right.$$

$$\left.+\frac{\left[2\omega_N+\omega_0^{(0)}\right]^2}{2\omega_N\left[\omega_N+\omega_0^{(0)}\right]}\right\}\cos(3\omega_N+2\omega_0)t$$

$$-\frac{3}{8}C_0\frac{F^4}{(\omega_N^2-\omega_0^2)^4}\left[4\omega_N-\omega_0^{(0)}\right]^2\left\{\left[\frac{\omega_N^2}{9\omega_N^2-\omega_0^{(0)2}}\right]+\frac{\left[2\omega_N-\omega_0^{(0)}\right]^2}{8\omega_N\left[\omega_N-\omega_0^{(0)}\right]}\right\}\cos(4\omega_N-\omega_0)t$$

$$-\frac{3}{8}C_0\frac{F^4}{(\omega_N^2-\omega_0^2)^4}\left[4\omega_N+\omega_0^{(0)}\right]^2\left\{\left[\frac{\omega_N^2}{9\omega_N^2-\omega_0^{(0)2}}\right]+\frac{\left[2\omega_N+\omega_0^{(0)}\right]^2}{8\omega_N\left[\omega_N+\omega_0^{(0)}\right]}\right\}\cos(4\omega_N+\omega_0)t$$

(S2.20)

As in the first-order correction, we must remove from (S2.20) the secular term proportional to $\cos\omega_0 t$. This defines the second-order frequency correction, viz.

$$\omega_0^{(2)}=\frac{9}{256}C_0^4\omega_0^{(0)}$$
$$+\frac{1}{32}C_0^2\frac{\omega_0^{(0)}F^2}{(\omega_N^2-\omega_0^2)^2}\left\{3+4\left[\frac{2\omega_N^2-\omega_0^{(0)2}}{\omega_N^2-\omega_0^{(0)2}}\right]+2\frac{\left[\omega_N-2\omega_0^{(0)}\right]^2}{\left[\omega_N-3\omega_0^{(0)}\right]\left[\omega_N-\omega_0^{(0)}\right]}\right.$$
$$\left.+2\frac{\left[\omega_N+2\omega_0^{(0)}\right]^2}{\left[\omega_N+\omega_0^{(0)}\right]\left[\omega_N+3\omega_0^{(0)}\right]}\right\}$$
$$+\frac{1}{32}\frac{\omega_0^{(0)}F^4}{(\omega_N^2-\omega_0^2)^4}\left\{3+4\left[\frac{\omega_N^2-2\omega_0^{(0)2}}{\omega_N^2-\omega_0^{(0)2}}\right]+\frac{\left[2\omega_N-\omega_0^{(0)}\right]^2}{4\omega_N\left[\omega_N-\omega_0^{(0)}\right]}+\frac{\left[2\omega_N+\omega_0^{(0)}\right]^2}{4\omega_N\left[\omega_N+\omega_0^{(0)}\right]}\right\}$$

(S2.21)

Upon removal of the secular term the integration of (S2.20) yields, with the aid of (S2.21), the result

$$A^{(2)}(t)=\frac{3}{64}C_0^3\left(\frac{25}{8}C_0^2\right.$$
$$+\frac{F^2}{(\omega_N^2-\omega_0^2)^2}\left\{4+\frac{3\left[\omega_N-2\omega_0^{(0)}\right]^2}{\left[\omega_N-3\omega_0^{(0)}\right]\left[\omega_N-\omega_0^{(0)}\right]}\right.$$
$$\left.\left.+\frac{3\left[\omega_N+2\omega_0^{(0)}\right]^2}{\left[\omega_N+\omega_0^{(0)}\right]\left[\omega_N+3\omega_0^{(0)}\right]}\right\}\right)\cos 3\omega_0 t+\frac{75}{3072}C_0^5\cos 5\omega_0 t$$

$$
\begin{aligned}
&+\frac{F}{\omega_N^2-\omega_0^2}\left(\frac{1}{16}C_0^4\left\{\frac{11}{8}\omega_0^{(0)2}-2\omega_N^2\left[\frac{2\omega_N^2-\omega_0^{(0)2}}{\omega_N^2-\omega_0^{(0)2}}\right]-\omega_N^2\frac{\left[\omega_N-2\omega_0^{(0)}\right]^2}{\left[\omega_N-3\omega_0^{(0)}\right]\left[\omega_N-\omega_0^{(0)}\right]}\right.\right.\\
&\qquad\left.-\omega_N^2\frac{\left[\omega_N+2\omega_0^{(0)}\right]^2}{\left[\omega_N+\omega_0^{(0)}\right]\left[\omega_N+3\omega_0^{(0)}\right]}\right\}\\
&\qquad+\frac{1}{16}C_0^2\frac{F^2}{(\omega_N^2-\omega_0^2)^2}\left\{4\omega_0^{(0)2}-\left[3\omega_N^2-4\omega_0^{(0)2}\right]\left[\frac{2\omega_N^2-\omega_0^{(0)2}}{\omega_N^2-\omega_0^{(0)2}}\right]-2\omega_N^2\left[\frac{\omega_N^2-2\omega_0^{(0)2}}{\omega_N^2-\omega_0^{(0)2}}\right]\right.\\
&\qquad+2\omega_0^{(0)2}\frac{\left[\omega_N-2\omega_0^{(0)}\right]^2}{\left[\omega_N-3\omega_0^{(0)}\right]\left[\omega_N-\omega_0^{(0)}\right]}+2\omega_0^{(0)2}\frac{\left[\omega_N+2\omega_0^{(0)}\right]^2}{\left[\omega_N+\omega_0^{(0)}\right]\left[\omega_N+3\omega_0^{(0)}\right]}\\
&\qquad\left.-\omega_N^2\frac{\left[2\omega_N-\omega_0^{(0)}\right]^2}{2\omega_N\left[\omega_N-\omega_0^{(0)}\right]}-\omega_N^2\frac{\left[2\omega_N+\omega_0^{(0)}\right]^2}{2\omega_N\left[\omega_N+\omega_0^{(0)}\right]}\right\}\\
&\qquad+\frac{1}{16}\frac{F^4}{(\omega_N^2-\omega_0^2)^4}\left\{4\omega_0^{(0)2}-\left[3\omega_N^2-4\omega_0^{(0)2}\right]\left[\frac{\omega_N^2-2\omega_0^{(0)2}}{\omega_N^2-\omega_0^{(0)2}}\right]+\omega_0^{(0)2}\frac{\left[2\omega_N-\omega_0^{(0)}\right]^2}{4\omega_N\left[\omega_N-\omega_0^{(0)}\right]}\right.\\
&\qquad\left.\left.+\omega_0^{(0)2}\frac{\left[2\omega_N+\omega_0^{(0)}\right]^2}{4\omega_N\left[\omega_N+\omega_0^{(0)}\right]}-3\omega_N^2\left[\frac{\omega_N^2}{9\omega_N^2-\omega_0^{(0)2}}\right]\right\}\right)\frac{\cos\omega_N t}{\omega_N^2-\omega_0^{(0)2}}
\end{aligned}
$$

$$
\begin{aligned}
&-\frac{9}{16}\frac{F^3}{(\omega_N^2-\omega_0^2)^3}\omega_N^2\left(C_0^2\left\{6\left[\frac{\omega_N^2}{9\omega_N^2-\omega_0^{(0)2}}\right]+\left[\frac{2\omega_N^2-\omega_0^{(0)2}}{\omega_N^2-\omega_0^{(0)2}}\right]+\frac{\left[2\omega_N-\omega_0^{(0)}\right]^2}{2\omega_N\left[\omega_N-\omega_0^{(0)}\right]}\right.\right.\\
&\qquad\left.+\frac{\left[2\omega_N+\omega_0^{(0)}\right]^2}{2\omega_N\left[\omega_N+\omega_0^{(0)}\right]}\right\}\\
&\qquad\left.+\frac{F^2}{(\omega_N^2-\omega_0^2)^2}\left\{6\left[\frac{\omega_N^2}{9\omega_N^2-\omega_0^{(0)2}}\right]+\left[\frac{\omega_N^2-2\omega_0^{(0)2}}{\omega_N^2-\omega_0^{(0)2}}\right]\right\}\right)\frac{\cos 3\omega_N t}{9\omega_N^2-\omega_0^{(0)2}}
\end{aligned}
$$

$$
-\frac{75}{16}\frac{F^5}{(\omega_N^2-\omega_0^2)^5}\left[\frac{\omega_N^4}{9\omega_N^2-\omega_0^{(0)2}}\right]\frac{\cos 5\omega_N t}{25\omega_N^2-\omega_0^{(0)2}}
$$

$$
+\frac{1}{16}C_0^2\frac{F}{\omega_N^2-\omega_0^2}\left(2\left[C_0^2+2\frac{F^2}{(\omega_N^2-\omega_0^2)^2}\right]\frac{\omega_0^{(0)}\left[\omega_N-2\omega_0^{(0)}\right]}{\left[\omega_N-\omega_0^{(0)}\right]\left[\omega_N-3\omega_0^{(0)}\right]}\right.
$$

$$
-C_0^2\frac{\left[\omega_N-2\omega_0^{(0)}\right]^2}{\left[\omega_N-\omega_0^{(0)}\right]\left[\omega_N-3\omega_0^{(0)}\right]}\left\{\frac{3}{4}+\left[\frac{2\omega_N^2-\omega_0^{(0)2}}{\omega_N^2-\omega_0^{(0)2}}\right]+2\frac{\left[\omega_N-2\omega_0^{(0)}\right]^2}{\left[\omega_N-3\omega_0^{(0)}\right]\left[\omega_N-\omega_0^{(0)}\right]}\right\}
$$

$$
-\frac{F^2}{(\omega_N^2-\omega_0^2)^2}\frac{\left[\omega_N-2\omega_0^{(0)}\right]^2}{\left[\omega_N-\omega_0^{(0)}\right]\left[\omega_N-3\omega_0^{(0)}\right]}\left\{\left[\frac{\omega_N^2-2\omega_0^{(0)2}}{\omega_N^2-\omega_0^{(0)2}}\right]+\frac{\left[2\omega_N-\omega_0^{(0)}\right]^2}{2\omega_N\left[\omega_N-\omega_0^{(0)}\right]}\right.
$$

$$
\left.\left.+2\frac{\left[\omega_N-2\omega_0^{(0)}\right]^2}{\left[\omega_N-3\omega_0^{(0)}\right]\left[\omega_N-\omega_0^{(0)}\right]}+\frac{\left[\omega_N+2\omega_0^{(0)}\right]^2}{\left[\omega_N+\omega_0^{(0)}\right]\left[\omega_N+3\omega_0^{(0)}\right]}\right\}\right)\cos(\omega_N-2\omega_0)t
$$

$$
-\frac{1}{16}C_0^2\frac{F}{\omega_N^2-\omega_0^2}\left(2\left[C_0^2+2\frac{F^2}{(\omega_N^2-\omega_0^2)^2}\right]\frac{\omega_0^{(0)}\left[\omega_N+2\omega_0^{(0)}\right]}{\left[\omega_N+\omega_0^{(0)}\right]\left[\omega_N+3\omega_0^{(0)}\right]}\right.
$$

$$
+C_0^2\frac{\left[\omega_N+2\omega_0^{(0)}\right]^2}{\left[\omega_N+\omega_0^{(0)}\right]\left[\omega_N+3\omega_0^{(0)}\right]}\left\{\frac{3}{4}+\left[\frac{2\omega_N^2-\omega_0^{(0)2}}{\omega_N^2-\omega_0^{(0)2}}\right]+2\frac{\left[\omega_N+2\omega_0^{(0)}\right]^2}{\left[\omega_N+\omega_0^{(0)}\right]\left[\omega_N+3\omega_0^{(0)}\right]}\right\}
$$

$$
+\frac{F^2}{(\omega_N^2-\omega_0^2)^2}\frac{\left[\omega_N+2\omega_0^{(0)}\right]^2}{\left[\omega_N+\omega_0^{(0)}\right]\left[\omega_N+3\omega_0^{(0)}\right]}\left\{\left[\frac{\omega_N^2-2\omega_0^{(0)2}}{\omega_N^2-\omega_0^{(0)2}}\right]+\frac{\left[2\omega_N+\omega_0^{(0)}\right]^2}{2\omega_N\left[\omega_N+\omega_0^{(0)}\right]}\right.
$$

$$
\left.\left.+2\frac{\left[\omega_N+2\omega_0^{(0)}\right]^2}{\left[\omega_N+\omega_0^{(0)}\right]\left[\omega_N+3\omega_0^{(0)}\right]}+\frac{\left[\omega_N-2\omega_0^{(0)}\right]^2}{\left[\omega_N-3\omega_0^{(0)}\right]\left[\omega_N-\omega_0^{(0)}\right]}\right\}\right)\cos(\omega_N+2\omega_0)t
$$

$$
-\frac{1}{16}C_0^4\frac{F}{\omega_N^2-\omega_0^2}\frac{\left[\omega_N-4\omega_0^{(0)}\right]^2}{\left[\omega_N-3\omega_0^{(0)}\right]\left[\omega_N-5\omega_0^{(0)}\right]}\left\{\frac{3}{4}+\frac{\left[\omega_N-2\omega_0^{(0)}\right]^2}{\left[\omega_N-3\omega_0^{(0)}\right]\left[\omega_N-\omega_0^{(0)}\right]}\right\}\cos(\omega_N-4\omega_0)t
$$

$$
-\frac{1}{16}C_0^4\frac{F}{\omega_N^2-\omega_0^2}\frac{\left[\omega_N+4\omega_0^{(0)}\right]^2}{\left[\omega_N+3\omega_0^{(0)}\right]\left[\omega_N+5\omega_0^{(0)}\right]}\left\{\frac{3}{4}+\frac{\left[\omega_N+2\omega_0^{(0)}\right]^2}{\left[\omega_N+\omega_0^{(0)}\right]\left[\omega_N+3\omega_0^{(0)}\right]}\right\}\cos(\omega_N+4\omega_0)t
$$

$$
-\frac{1}{16}C_0\frac{F^2}{(\omega_N^2-\omega_0^2)^2}\left(\left[C_0^2+2\frac{F^2}{(\omega_N^2-\omega_0^2)^2}\right]\frac{\omega_1^{(0)}\left[2\omega_N-\omega_0^{(0)}\right]}{4\omega_N\left[\omega_N-\omega_0^{(0)}\right]}\right.
$$

$$
-C_0^2\frac{\left[2\omega_N-\omega_0^{(0)}\right]^2}{2\omega_N\left[\omega_N-\omega_0^{(0)}\right]}\left\{\left[\frac{2\omega_N^2-\omega_0^{(0)2}}{\omega_N^2-\omega_0^{(0)2}}\right]+\frac{\left[\omega_N-2\omega_0^{(0)}\right]^2}{\left[\omega_N-3\omega_0^{(0)}\right]\left[\omega_N-\omega_0^{(0)}\right]}\right.
$$

$$
\left.+\frac{\left[2\omega_N-\omega_0^{(0)}\right]^2}{4\omega_N\left[\omega_N-\omega_0^{(0)}\right]}+\frac{\left[2\omega_N+\omega_0^{(0)}\right]^2}{8\omega_N\left[\omega_N+\omega_0^{(0)}\right]}\right\}
$$

$$
-\frac{F^2}{(\omega_N^2-\omega_0^2)^2}\frac{\left[2\omega_N-\omega_0^{(0)}\right]^2}{2\omega_N\left[\omega_N-\omega_0^{(0)}\right]}\left\{\left[\frac{\omega_N^2-2\omega_0^{(0)2}}{\omega_N^2-\omega_0^{(0)2}}\right]+3\left[\frac{\omega_N^2}{9\omega_N^2-\omega_0^{(0)2}}\right]\right.
$$

$$
\left.\left.+\frac{\left[2\omega_N-\omega_0^{(0)}\right]^2}{4\omega_N\left[\omega_N-\omega_0^{(0)}\right]}\right\}\right)\cos(2\omega_N-\omega_0)t
$$

$$
+\frac{1}{16}C_0\frac{F^2}{(\omega_N^2-\omega_0^2)^2}\left(\left[C_0^2+2\frac{F^2}{(\omega_N^2-\omega_0^2)^2}\right]\frac{\omega_0^{(0)}\left[2\omega_N+\omega_0^{(0)}\right]}{4\omega_N\left[\omega_N+\omega_0^{(0)}\right]}\right.
$$

$$
+C_0^2\frac{\left[2\omega_N+\omega_0^{(0)}\right]^2}{2\omega_N\left[\omega_N+\omega_0^{(0)}\right]}\left\{\left[\frac{2\omega_N^2-\omega_0^{(0)2}}{\omega_N^2-\omega_0^{(0)2}}\right]+\frac{\left[\omega_N+2\omega_0^{(0)}\right]^2}{\left[\omega_N+\omega_0^{(0)}\right]\left[\omega_N+3\omega_0^{(0)}\right]}\right.
$$

$$
\left.+\frac{\left[2\omega_N+\omega_0^{(0)}\right]^2}{4\omega_N\left[\omega_N+\omega_0^{(0)}\right]}+\frac{\left[2\omega_N-\omega_0^{(0)}\right]^2}{8\omega_N\left[\omega_N-\omega_0^{(0)}\right]}\right\}
$$

$$
+\frac{F^2}{(\omega_N^2-\omega_0^2)^2}\frac{\left[2\omega_N+\omega_0^{(0)}\right]^2}{2\omega_N\left[\omega_N+\omega_0^{(0)}\right]}\left\{\left[\frac{\omega_N^2-2\omega_0^{(0)2}}{\omega_N^2-\omega_0^{(0)2}}\right]+3\left[\frac{\omega_N^2}{9\omega_N^2-\omega_0^{(0)2}}\right]\right.
$$

$$
\left.\left.+\frac{\left[2\omega_N+\omega_0^{(0)}\right]^2}{4\omega_N\left[\omega_N+\omega_0^{(0)}\right]}\right\}\right)\cos(2\omega_N+\omega_0)t
$$

$$
+\frac{1}{256}C_0^3\frac{F^2}{(\omega_N^2-\omega_0^2)^2}\frac{\left[2\omega_N-3\omega_0^{(0)}\right]^2}{\left[\omega_N-\omega_0^{(0)}\right]\left[\omega_N-2\omega_0^{(0)}\right]}\left\{\frac{3}{2}+\frac{\left[2\omega_N-\omega_0^{(0)}\right]^2}{\omega_N\left[\omega_N-\omega_0^{(0)}\right]}\right.
$$

$$
\left.+2\frac{\left[\omega_N-2\omega_0^{(0)}\right]^2}{\left[\omega_N-3\omega_0^{(0)}\right]\left[\omega_N-\omega_0^{(0)}\right]}\right\}\cos(2\omega_N-3\omega_0)t
$$

$$+\frac{1}{256}C_0^3\frac{F^2}{(\omega_N^2-\omega_0^2)^2}\frac{\left[2\omega_N+3\omega_0^{(0)}\right]^2}{\left[\omega_N+\omega_0^{(0)}\right]\left[\omega_N+2\omega_0^{(0)}\right]}\left\{\frac{3}{2}+\frac{\left[2\omega_N+\omega_0^{(0)}\right]^2}{\omega_N\left[\omega_N+\omega_0^{(0)}\right]}\right.$$

$$\left.+2\frac{\left[\omega_N+2\omega_0^{(0)}\right]^2}{\left[\omega_N+\omega_0^{(0)}\right]\left[\omega_N+3\omega_0^{(0)}\right]}\right\}\cos(2\omega_N+3\omega_0)t$$

$$-\frac{1}{48}C_0^2\frac{F^3}{(\omega_N^2-\omega_0^2)^3}\frac{\left[3\omega_N-2\omega_0^{(0)}\right]^2}{\left[3\omega_N-\omega_0^{(0)}\right]\left[\omega_N-\omega_0^{(0)}\right]}\left\{3\left[\frac{\omega_N^2}{9\omega_N^2-\omega_0^{(0)2}}\right]+\frac{\left[\omega_N-2\omega_0^{(0)}\right]^2}{\left[\omega_N-3\omega_0^{(0)}\right]\left[\omega_N-\omega_0^{(0)}\right]}\right.$$

$$\left.+\frac{\left[2\omega_N-\omega_0^{(0)}\right]^2}{2\omega_N\left[\omega_N-\omega_0^{(0)}\right]}\right\}\cos(3\omega_N-2\omega_0)t$$

$$-\frac{1}{48}C_0^2\frac{F^3}{(\omega_N^2-\omega_0^2)^3}\frac{\left[3\omega_N+2\omega_0^{(0)}\right]^2}{\left[3\omega_N+\omega_0^{(0)}\right]\left[\omega_N+\omega_0^{(0)}\right]}\left\{3\left[\frac{\omega_N^2}{9\omega_N^2-\omega_0^{(0)2}}\right]+\frac{\left[\omega_N+2\omega_0^{(0)}\right]^2}{\left[\omega_N+\omega_0^{(0)}\right]\left[\omega_N+3\omega_0^{(0)}\right]}\right.$$

$$\left.+\frac{\left[2\omega_N+\omega_0^{(0)}\right]^2}{2\omega_N\left[\omega_N+\omega_0^{(0)}\right]}\right\}\cos(3\omega_N+2\omega_0)t$$

$$+\frac{3}{64}C_0\frac{F^4}{(\omega_N^2-\omega_0^2)^4}\frac{\left[4\omega_N-\omega_0^{(0)}\right]^2}{\omega_N\left[2\omega_N-\omega_0^{(0)}\right]}\left\{\frac{\omega_N^2}{9\omega_N^2-\omega_0^{(0)2}}+\frac{\left[2\omega_N-\omega_0^{(0)}\right]^2}{8\omega_N\left[\omega_N-\omega_0^{(0)}\right]}\right\}\cos(4\omega_N-\omega_0)t$$

$$+\frac{3}{64}C_0\frac{F^4}{(\omega_N^2-\omega_0^2)^4}\frac{\left[4\omega_N+\omega_0^{(0)}\right]^2}{\omega_N\left[2\omega_N+\omega_0^{(0)}\right]}\left\{\frac{\omega_N^2}{9\omega_N^2-\omega_0^{(0)2}}+\frac{\left[2\omega_N+\omega_0^{(0)}\right]^2}{8\omega_N\left[\omega_N+\omega_0^{(0)}\right]}\right\}\cos(4\omega_N+\omega_0)t$$

(S2.22)

Equations (S2.21) and (S2.22) constitute the second-order corrections.

## Approximate Solution to Second Order

The approximate solution to second order in $\epsilon$ of the amplitude $A(t)$ is the sum of the corrections given by (S2.8), (S2.16), and (S2.22), i.e., $A(t) \cong A^{(0)}(t) + A^{(1)}(t) + A^{(2)}(t)$, where we now set $\epsilon = 1$. Note from (S2.22) that we now have third and fifth harmonics of both $\omega_0$ and $\omega_N$ appearing in the solution, but there are no even harmonics of these frequencies. Figure S2.1, below, depicts a sketch of the frequency output in second order of the successive approximation expansion. Again, we see the beginning of sidebands around each pump harmonic, including the even harmonics of frequency $2\omega_N$ and $4\omega_N$, even though the corresponding amplitudes of these specific frequencies themselves do not appear in the output spectrum. The FSR is clearly twice the fundamental frequency $\omega_0$ and, as mentioned earlier, the sidebands of the odd (even) pump harmonics fill in at even (odd) multiples of the fundamental frequency, with respect to the principle peak of each. Again, the selection rules

determining which sideband teeth appear have their origin in the symmetry of the film geometry, owing to the terms that appear in the expansion of the kinetic inductance of (S2.1).

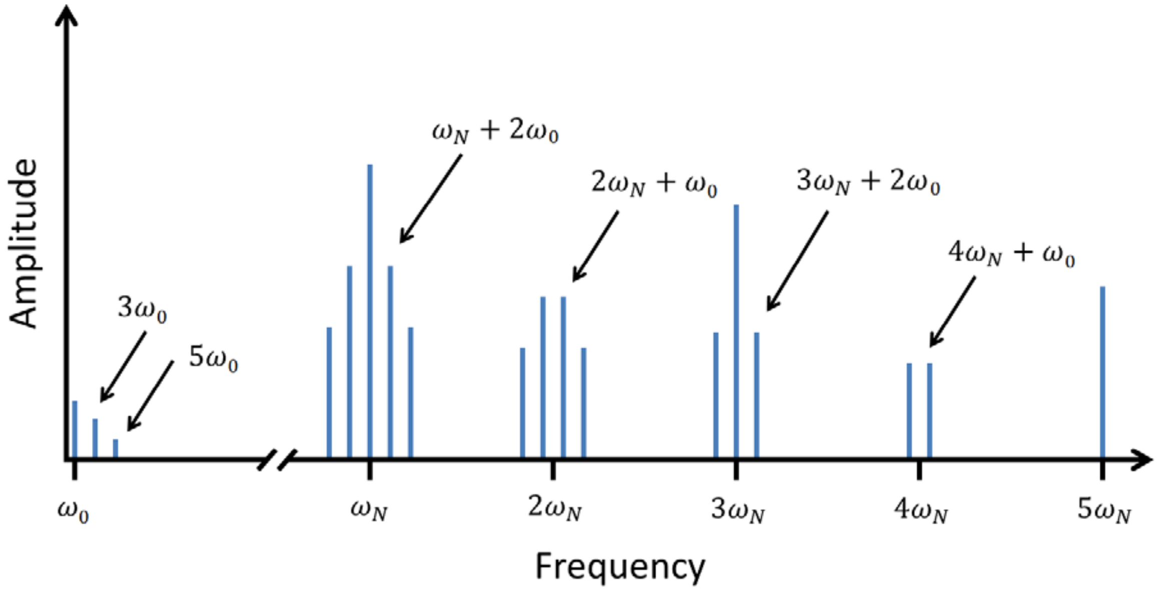


**Figure S2.1.** Sketch depicting the frequency spectrum of the output current, as obtained from second-order perturbation theory.

In the second order approximation the renormalized fundamental frequency is given by (S2.15) and (S2.21) applied to (S2.5). If the pump tone is situated at sufficiently large $N$ such that $\omega_N^2 \gg \omega_0^{(0)2}$ then the frequency may be expressed as

$$\omega_0 \cong \omega_0^{(0)} \left[ 1 - \frac{1}{8}\left( C_0^2 + 2\frac{F^2}{\omega_N^4} \right) + \frac{3}{256}\left( 3C_0^4 + 40C_0^2 \frac{F^2}{\omega_N^4} + 24\frac{F^4}{\omega_N^8} \right) \right] \tag{S2.23}$$

The coefficient $C_0$ must still be determined.

Note that the initial boundary condition $\dot{A}(0) = 0$ is satisfied by our approximation $A(t) \cong A^{(0)}(t) + A^{(1)}(t) + A^{(2)}(t)$. To satisfy $A(0) = 0$ we set the value of the constant $C_0$ via $A^{(0)}(0) + A^{(1)}(0) + A^{(2)}(0) = 0$. This condition produces a polynomial in powers of $C_0$ whose roots are the possible solutions for the constant. Assuming $C_0$ evolves continuously and only modestly from its zero-order value of $F/(\omega_N^2 - \omega_0^2) \cong F/\omega_N^2$ we may express the solution as an expansion in powers of $F/\omega_N^2$. To estimate (S2.23) to fourth power in $F/\omega_N^2$ we need only consider an approximation of $C_0$ to third power. It is then sufficient to estimate $C_0$ via $A^{(0)}(0) + A^{(1)}(0) \cong 0$ since $A^{(2)}(0)$ contributes only terms of order five and higher. Thus, from (S2.8) and (S2.16) we obtain

$$\frac{3}{32}C_0^3-\frac{F}{\omega_N^2}C_0^2-\left(1-\frac{1}{2}\frac{F^2}{\omega_N^4}\right)C_0-\frac{1}{3}\frac{F^3}{\omega_N^6}+\frac{F}{\omega_N^2}\cong 0$$

(S2.24)

The solution of $C_0$ via (S2.24) determines the shifted fundamental frequency of (S2.23). Specifically, writing $C_0=\alpha_1\,F/\omega_N^2+\alpha_2\,F^2/\omega_N^4+\alpha_3\,F^3/\omega_N^6+\cdots$ and applying this expansion to (S2.24) we find

$$C_0\cong\frac{F}{\omega_N^2}-\frac{71}{96}\frac{F^3}{\omega_N^6},\qquad F/\omega_N^2\ll 1$$

(S2.25)

such that

$$\omega_0\cong\omega_0^{(0)}\left(1-\frac{3}{8}\frac{F^2}{\omega_N^4}+\frac{745}{768}\frac{F^4}{\omega_N^8}\right),\qquad F/\omega_N^2\ll 1$$

(S2.26)

# Supplement 3: Device Fabrication

The device used in this work consisted of a 25 cm long, double-spiral, λ/2 resonator made from a 2/2 μm wide center-electrode/gap coplanar waveguide (CPW) on intrinsic Si (>20 kOhm-cm). See Figure S3.1, below. The CPW was fabricated from a film of superconducting material that was patterned using optical lithography. A single step, $SF_6$ reactive ion etch was used to process the film in order to minimize loss.[4] The film was comprised of 20 nm niobium titanium nitride ($Nb_{0.7}Ti_{0.3}N$) that was deposited at 500 $^oC$ using reactive co-sputtering from niobium and titanium targets in an $Ar:N_2$ atmosphere. It had a

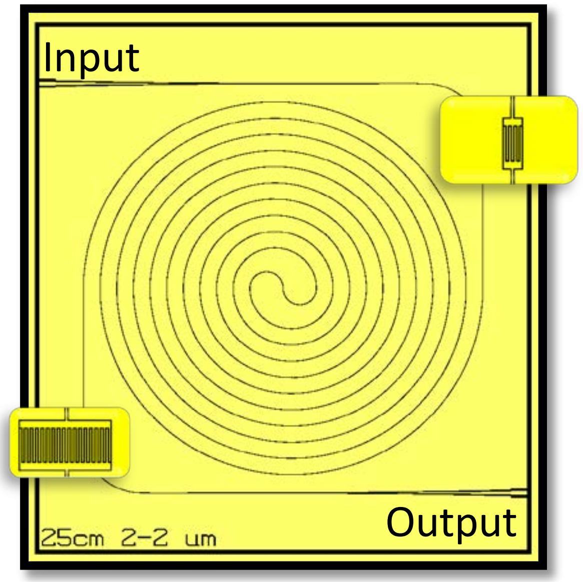


**Figure S3.1.** Layout of 20 x 20 mm frequency comb chip with 25 cm long double spiral resonator. The inter-digitated capacitors (insets) on the input and output are 16 and 180 fF, respectively. They are connected micorowave launch with an exponential impedance matching taper that transforms the Z=50 ohm 200-80 μm width-gap CPW launch to a Z=120 ohm 2-2 μm CPW. The light areas are superconducting NbTiN, the gap is shown dark.

critical temperature $T_C$ = 13.8 K, and measurements were conducted at relatively low temperatures, from 0.05K < T < 6 K. No frequency dispersion was observed in transmission line test structures of the NbTiN from DC up to at least 20 GHz. This can be expected to be the case up to frequencies comparable to twice the superconducting gap, i.e. $f \sim 2\Delta/h = 2\times 1.76 k_B T_C/h \sim 1$ *THz.*

The fundamental resonator frequency was measured to be $f_o$ =59.738181 MHz, in good agreement with that expected from the formula $f_0 = \sqrt{1-\alpha}\frac{c}{2ln_{eff}}$ where the length of the CPW resonator is *l*=0.25 m, the effective dielectric constant is $n_{eff}$=2.6 for a CPW on Si, and the kinetic inductance fraction $\alpha = 0.93$ was determined from the frequency shift of a test resonator. It agrees well with the value obtained from Mattis-Bardeen theory using the measured sheet resistance of 84 Ω/square, giving a value for the kinetic inductance of $L_0$ =6 pH/square. The nonlinearity of the total inductance, given by equation (S2.1), was observed to be up to $[I_0^{Max}(t)/I_*]^2$ = 9%, where the scaling factor $I_* = 12\,mA$ is

on the order of the superconductor critical current. Values of the coupling capacitors on the input and output of 16 and 180 fF were chosen to be critically coupled at 5 GHz and 100 MHz, respectively, in order to pump the system optimally at high frequency and allow low frequency energy out.

# References

[1] M. E. Levinson, J. Appl. Phys. **20**, 1045 (1949); C. Holmes and P. Holmes, J. of Sound and Vibration **78** (2), 161 (1981)

[2] D. W. Jordan and P. Smith, *Nonlinear Ordinary Differential Equations: An Introduction for Scientists and Engineers*, (Oxford University Press, Oxford, 2007), Fourth Edition, pp. 242-251.

[3] L. D. Landau and E. M. Lifshitz, *Mechanics*, (Pergamon Press, Oxford, 1976), Third Edition, pp. 84-92.

[4] P. Del'Hay, O. Arcizet, A. Schliesser, R. Holzwarth, T.J. Kippenberg, Phys. Rev. Lett. **101,** 053903 (2008).

*David.P.Pappas@NIST.gov
